# Supplementary material for: Microhartree Precision in Density-Functional-Theory Calculations
Source: arXiv:1803.00776 source file (2018-03-02)
Supplement: Supplementary file 1 [file supplemental.pdf]

# Microhartree Precision in Density-Functional-Theory Calculations
# Supplemental Material

Andris Gulans[1], Anton Kozhevnikov[2], and Claudia Draxl[1]
[1] *Physics Department and IRIS Adlershof, Humboldt-Universität zu Berlin, Zum Großen Windkanal 6, 12489 Berlin, Germany and*
[2] *Swiss National Supercomputing Center, Lugano, Switzerland*
(Dated: November 13, 2017)

## I. TOTAL ENERGY CALCULATIONS

### A. exciting calculations

The total-energy calculations of atoms are performed with **exciting**[1] using atomic-sphere radii of $R_{\mathrm{MT}}$=1.2 bohr for all elements. The computational settings which correspond to the basis-set limit and non-interacting isolated atoms are summarized together with the corresponding total energies in Table I.

The calculations of molecules are performed with the same LO basis as described above. Other computational parameters are specified in Tables II–III. These settings correspond to total energies converged to the sub-$\mu$Ha level for each molecule. The obtained total energies, $E^{\mathrm{tot}}$, and atomization energies, $E^{\mathrm{at}}$, are given in Table III. The atomization energy of a molecule is defined as $E^{\mathrm{at}} = E^{\mathrm{tot}} - \sum_{\alpha} N_{\alpha} E_{\alpha}$, where $N_{\alpha}$ is the number of atoms of each kind in the molecule, and $E_{\alpha}$ is the total energy of the corresponding isolated atom. Despite the mismatch between the computational parameters in calculations of atoms and molecules, $E_{\alpha}$ are always taken from Table I, since the converged limit has been reached.

TABLE I. Absolute total energies of atoms, $E$, calculated with **exciting** and employed computational settings: dimensionless planewave cutoff, $R_{\mathrm{MT}}G_{\mathrm{max}}$, local-orbital (LO) basis, and size of the unit cell, $d$. The description of the LO basis indicates how many LOs of each $\ell m$ channel are used.

| Atom | $R_{\mathrm{MT}}G_{\mathrm{max}}$ | LO basis | $d$ [a.u.] | $E$ [Ha] |
|---|---|---|---|---|
| H | 10 | $2s\,2p\,1d$ | 35 | -0.4787107 |
| He | 12 | $4s\,2p\,2d$ | 35 | -2.8344552 |
| Li | 12 | $4s\,2p\,2d$ | 40 | -7.3432843 |
| Be | 12 | $5s\,2p\,2d$ | 35 | -14.4464735 |
| B | 12 | $5s\,5p\,7d\,4f\,3g\,3h$ | 35 | -24.3548568 |
| C | 12 | $5s\,5p\,7d\,4f\,3g\,3h$ | 35 | -37.4685404 |
| N | 12 | $5s\,5p\,7d\,4f\,3g\,3h$ | 35 | -54.1343867 |
| O | 13 | $5s\,5p\,7d\,4f\,3g\,3h$ | 35 | -74.5286993 |
| F | 13 | $5s\,5p\,7d\,4f\,3g\,3h$ | 35 | -99.1118530 |
| Ne | 13 | $5s\,5p\,7d\,4f\,3g\,3h$ | 35 | -128.2299171 |
| Na | 13 | $4s\,4p\,5d\,5f\,2g$ | 40 | -161.4436320 |
| Mg | 13 | $4s\,4p\,5d\,5f\,2g$ | 35 | -199.1352882 |
| Al | 13 | $4s\,4p\,5d\,5f\,2g$ | 45 | -241.3178300 |
| Si | 13 | $4s\,4p\,5d\,5f\,2g$ | 40 | -288.2171655 |
| P | 14 | $4s\,4p\,5d\,5f\,2g$ | 35 | -340.0000526 |
| S | 14 | $4s\,4p\,5d\,5f\,2g$ | 35 | -396.7390648 |
| Cl | 14 | $4s\,4p\,5d\,5f\,2g$ | 35 | -458.6643433 |
| Ar | 14 | $4s\,4p\,5d\,5f\,2g$ | 40 | -525.9397933 |

TABLE II. Computational parameters used in the calculation of the molecules of the G2-1 set.

| Atom | $R_{\mathrm{MT}}G_{\mathrm{max}}$ | $R_{\mathrm{MT}}$ [a.u.] | Atom | $R_{\mathrm{MT}}G_{\mathrm{max}}$ | $R_{\mathrm{MT}}$ [a.u.] |
|---|---|---|---|---|---|
| H | 9.0 | 0.7–1.2 | F | 12.0–13.0 | 1.0–1.2 |
| Li | 12.0 | 1.2–1.5 | Na | 13.0 | 1.5 |
| Be | 12.0 | 1.2 | Si | 12.6–14.0 | 1.2–1.4 |
| C | 12.0–12.9 | 1.0–1.2 | P | 12.6–13.0 | 1.2–1.4 |
| N | 12.0–12.9 | 1.0 | S | 12.6–14.0 | 1.0–1.5 |
| O | 12.0–13.0 | 1.0–1.2 | Cl | 12.6–14.1 | 1.0–1.5 |

TABLE III. Total and atomization energies ($E^{\mathrm{tot}}$ and $E^{\mathrm{at}}$) of G2-1 molecules obtained with `exciting` and unit-cell size, $d$.

| Molecule | $d$ [a.u.] | $E^{\mathrm{tot}}$ [Ha] | $E^{\mathrm{at}}$ [Ha] | Molecule | $d$ [a.u.] | $E^{\mathrm{tot}}$ [Ha] | $E^{\mathrm{at}}$ [Ha] |
|---|---|---|---|---|---|---|---|
| LiH | 40 | -7.9189095 | -0.0969145 | CO | 35 | -112.4738244 | -0.4765847 |
| BeH | 35 | -15.0211314 | -0.0959472 | HCO | 35 | -113.0066196 | -0.5306692 |
| CH | 35 | -38.0946520 | -0.1474009 | $H_2CO$ | 35 | -113.6460326 | -0.6913715 |
| $CH_2$ ($^3B_1$) | 35 | -38.7647945 | -0.3388328 | $CH_3OH$ | 35 | -114.8464907 | -0.9344083 |
| $CH_2$ ($^1A_1$) | 30 | -38.7429684 | -0.3170066 | $N_2$ | 25 | -108.6955437 | -0.4267704 |
| $CH_3$ | 35 | -39.4449793 | -0.5403068 | $H_2NN_2H$ | 35 | -111.0058791 | -0.8222630 |
| $CH_4$ | 35 | -40.1199025 | -0.7365194 | NO | 35 | -128.9801855 | -0.3170996 |
| NH | 35 | -54.7652713 | -0.1521740 | $O_2$ | 35 | -149.3363030 | -0.2789045 |
| $NH_2$ | 35 | -55.4233623 | -0.3315543 | $H_2O_2$ | 35 | -150.5490116 | -0.5341917 |
| $NH_3$ | 30 | -56.1081309 | -0.5376121 | $F_2$ | 30 | -198.3482928 | -0.1245868 |
| OH | 35 | -75.2053260 | -0.1979161 | $CO_2$ | 35 | -187.2799890 | -0.7540500 |
| $H_2O$ | 30 | -75.9108608 | -0.4247401 | $Na_2$ | 45 | -322.9197317 | -0.0324677 |
| HF | 20 | -99.8490047 | -0.2584410 | $Si_2$ | 40 | -576.5831389 | -0.1488079 |
| $SiH_2$ ($^1A_1$) | 35 | -289.4396362 | -0.2650493 | $P_2$ | 35 | -680.2298843 | -0.2297791 |
| $SiH_2$ ($^3B_1$) | 35 | -289.4088326 | -0.2342457 | $S_2$ | 35 | -793.6938121 | -0.2156825 |
| $SiH_3$ | 35 | -290.0464654 | -0.3931678 | $Cl_2$ | 35 | -917.4606552 | -0.1319686 |
| $SiH_4$ | 35 | -290.6853928 | -0.5533845 | NaCl | 40 | -620.2737537 | -0.1657784 |
| $PH_2$ | 35 | -341.2347271 | -0.2772531 | SiO | 35 | -363.1037326 | -0.3578678 |
| $PH_3$ | 35 | -341.8665211 | -0.4303364 | CS | 35 | -434.5299351 | -0.3223299 |
| $SH_2$ | 35 | -398.0257197 | -0.3292335 | OS | 35 | -471.5346930 | -0.2669289 |
| HCl | 35 | -459.3350394 | -0.1919854 | ClO | 35 | -533.3579909 | -0.1649483 |
| $Li_2$ | 45 | -14.7244547 | -0.0378862 | ClF | 35 | -557.9276308 | -0.1514345 |
| LiF | 30 | -106.7043526 | -0.2492153 | $Si_2H_6$ | 40 | -580.2300293 | -0.9234342 |
| $C_2H_2$ | 35 | -76.6276624 | -0.7331602 | $CH_3Cl$ | 35 | -498.2811348 | -0.7121190 |
| $C_2H_4$ | 35 | -77.8596989 | -1.0077753 | $CH_3SH$ | 35 | -436.9771630 | -0.8547150 |
| $C_2H_6$ | 35 | -79.0742387 | -1.2648938 | HOCl | 35 | -534.0077637 | -0.3360104 |
| CN | 35 | -91.9531185 | -0.3501915 | $SO_2$ | 35 | -546.3326934 | -0.5362301 |
| HCN | 35 | -92.6569957 | -0.5753580 | | | | |

### B. NWChem calculations

NWChem[2] calculations of atoms are performed using an uncontracted even-tempered Gaussian basis set consisting of 44 *s*-, 29 *p*-, 15 *d*-, 13 *f*-, 13 *g*-, 9 *h*- and 4 *i*-type shells for each atom. In case of molecules, the `aug-cc-pVQZ` basis set is employed for Li, Be and Na, while the `aug-cc-pV5Z` basis set is used for all remaining atoms. `aug-cc-pVQZ` and `aug-cc-pV5Z`[3] are considerably less accurate and, thus, incompatible with the even-tempered basis sets. Therefore, the evaluation of the atomization energies requires that the energies of individual atoms are obtained employing exactly the same basis set as in the calculation of molecules. The obtained results are given in Table IV.

The original implementation of NWChem uses the modified Perdew-Wang parametrization of the local-density approximation. Therefore, we have introduced changes in the source code, according to the original definition in Ref. 4 in order to make it consistent with the calculations carried out with **exciting** and MADNESS.

TABLE IV. Total and atomization energies ($E^{\text{tot}}$ and $E^{\text{at}}$) of G2-1 molecules obtained with NWChem.

| Molecule | $E^{\text{tot}}$ [Ha] | $E^{\text{at}}$ [Ha] | Molecule | $E^{\text{tot}}$ [Ha] | $E^{\text{at}}$ [Ha] |
|---|---|---|---|---|---|
| LiH | -7.9186098 | -0.0971543 | CO | -112.4732620 | -0.4765927 |
| BeH | -15.0207205 | -0.0962214 | HCO | -113.0060522 | -0.5306776 |
| CH | -38.0944580 | -0.1474132 | $H_2CO$ | -113.6454703 | -0.6913904 |
| $CH_2$ ($^3B_1$) | -38.7645931 | -0.3388429 | $CH_3OH$ | -114.8459379 | -0.9344474 |
| $CH_2$ ($^1A_1$) | -38.7427588 | -0.3170086 | $N_2$ | -108.6949952 | -0.4267559 |
| $CH_3$ | -39.4447687 | -0.5403131 | $H_2NN_2H$ | -111.0053582 | -0.8222977 |
| $CH_4$ | -40.1196937 | -0.7365329 | NO | -128.9795605 | -0.3171112 |
| NH | -54.7650189 | -0.1521939 | $O_2$ | -149.3355799 | -0.2789204 |
| $NH_2$ | -55.4231050 | -0.3315747 | $H_2O_2$ | -150.5483170 | -0.5342469 |
| $NH_3$ | -56.1078590 | -0.5376234 | $F_2$ | -198.3473901 | -0.1246221 |
| OH | -75.2049730 | -0.1979379 | $CO_2$ | -187.2790659 | -0.7540669 |
| $H_2O$ | -75.9105054 | -0.4247650 | $Na_2$ | -322.9044918 | -0.0334341 |
| HF | -99.8485534 | -0.2584641 | $Si_2$ | -576.5710246 | -0.1444462 |
| $SiH_2$ ($^1A_1$) | -289.4357265 | -0.2650266 | $P_2$ | -680.2221879 | -0.2295684 |
| $SiH_2$ ($^3B_1$) | -289.4049636 | -0.2342638 | $S_2$ | -793.6860562 | -0.2153452 |
| $SiH_3$ | -290.0425712 | -0.3931660 | $Cl_2$ | -917.4527318 | -0.1317304 |
| $SiH_4$ | -290.6814615 | -0.5533510 | NaCl | -620.2613629 | -0.1653333 |
| $PH_2$ | -341.2309447 | -0.2772243 | SiO | -363.0991175 | -0.3574985 |
| $PH_3$ | -341.8627265 | -0.4303008 | CS | -434.5258431 | -0.3221480 |
| $SH_2$ | -398.0219341 | -0.3291679 | OS | -471.5301190 | -0.2664338 |
| HCl | -459.3311780 | -0.1919720 | ClO | -533.3534435 | -0.1646131 |
| $Li_2$ | -14.7236351 | -0.0381346 | ClF | -557.9230973 | -0.1512126 |
| LiF | -106.7034041 | -0.2492699 | $Si_2H_6$ | -580.2222366 | -0.9234263 |
| $C_2H_2$ | -76.6272481 | -0.7331583 | $CH_3Cl$ | -498.2770578 | -0.7121016 |
| $C_2H_4$ | -77.8592878 | -1.0077874 | $CH_3SH$ | -436.9731605 | -0.8546441 |
| $C_2H_6$ | -79.0738403 | -1.2649293 | HOCl | -534.0034010 | -0.3358653 |
| CN | -91.9526478 | -0.3501886 | $SO_2$ | -546.3262974 | -0.5342824 |
| HCN | -92.6565270 | -0.5753625 | | | |

### C. MADNESS calculations

MADNESS calculations involve only a few computational parameters: the convergence thresholds for the total energy and electron density as well as the *control* parameter. Both thresholds are set to $10^{-7}$ a.u., while the *control* parameter is set to $10^{-8}$. The results of G2-1 calculations are given in Table V.

TABLE V. Total and atomization energies ($E^{\text{tot}}$ and $E^{\text{at}}$) of G2-1 molecules obtained with MADNESS.

| Molecule | $E^{\text{tot}}$ [Ha] | $E^{\text{at}}$ [Ha] | Molecule | $E^{\text{tot}}$ [Ha] | $E^{\text{at}}$ [Ha] |
|---|---|---|---|---|---|
| LiH | -7.9189088 | -0.0969157 | CO | -112.4738240 | -0.4765855 |
| BeH | -15.0211313 | -0.0959480 | HCO | -113.0066185 | -0.5306695 |
| CH | -38.0946508 | -0.1474009 | $H_2CO$ | -113.6460315 | -0.6913722 |
| $CH_2$ ($^3B_1$) | -38.7647924 | -0.3388321 | $CH_3OH$ | -114.8464901 | -0.9344100 |
| $CH_2$ ($^1A_1$) | -38.7429677 | -0.3170074 | $N_2$ | -108.6955432 | -0.4267713 |
| $CH_3$ | -39.4449785 | -0.5403078 | $H_2NN_2H$ | -111.0058779 | -0.8222643 |
| $CH_4$ | -40.1199017 | -0.7365206 | NO | -128.9801849 | -0.3170998 |
| NH | -54.7652705 | -0.1521741 | $O_2$ | -149.3363028 | -0.2789047 |
| $NH_2$ | -55.4233615 | -0.3315547 | $H_2O_2$ | -150.5490116 | -0.5341927 |
| $NH_3$ | -56.1081301 | -0.5376129 | $F_2$ | -198.3482931 | -0.1245864 |
| OH | -75.2053253 | -0.1979159 | $CO_2$ | -187.2799858 | -0.7540482 |
| $H_2O$ | -75.9108601 | -0.4247403 | $Na_2$ | -322.9197298 | -0.0324700 |
| HF | -99.8490035 | -0.2584397 | $Si_2$ | -576.5831375 | -0.1488097 |
| $SiH_2$ ($^1A_1$) | -289.4396367 | -0.2650520 | $P_2$ | -680.2298837 | -0.2297821 |
| $SiH_2$ ($^3B_1$) | -289.4088311 | -0.2342465 | $S_2$ | -793.6938128 | -0.2156846 |
| $SiH_3$ | -290.0464643 | -0.3931692 | $Cl_2$ | -917.4606565 | -0.1319701 |
| $SiH_4$ | -290.6853924 | -0.5533869 | NaCl | -620.2737531 | -0.1657800 |
| $PH_2$ | -341.2347274 | -0.2772558 | SiO | -363.1037323 | -0.3578693 |
| $PH_3$ | -341.8665221 | -0.4303402 | CS | -434.5299353 | -0.3223316 |
| $SH_2$ | -398.0257212 | -0.3292363 | OS | -471.5346934 | -0.2669302 |
| HCl | -459.3350406 | -0.1919870 | ClO | -533.3579908 | -0.1649485 |
| $Li_2$ | -14.7244534 | -0.0378880 | ClF | -557.9276321 | -0.1514355 |
| LiF | -106.7043529 | -0.2492169 | $Si_2H_6$ | -580.2300286 | -0.9234384 |
| $C_2H_2$ | -76.6276616 | -0.7331617 | $CH_3Cl$ | -498.2811345 | -0.7121206 |
| $C_2H_4$ | -77.8596981 | -1.0077775 | $CH_3SH$ | -436.9771635 | -0.8547183 |
| $C_2H_6$ | -79.0742376 | -1.2648962 | HOCl | -534.0077643 | -0.3360117 |
| CN | -91.9531176 | -0.3501921 | $SO_2$ | -546.3326930 | -0.5362308 |
| HCN | -92.6569951 | -0.5753592 | | | |

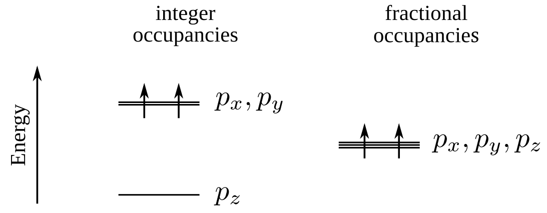


FIG. 1. Schematic of atomic silicon-$3p$ levels for the majority-spin channel in LSDA calculations with the arrows indicating the occupation.

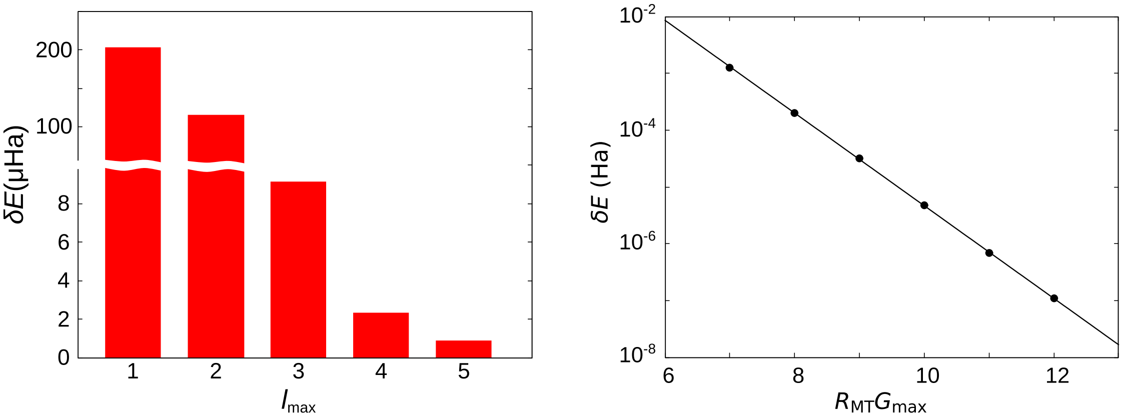


FIG. 2. Error in the total GGA energy of an oxygen atom when using local orbitals with angular momenta up to $\ell_{\max}$ (left) and as a function of a planewave cutoff $R_{\mathrm{MT}}G_{\max}$ (right). The limit of the total energy is estimated by using $\ell_{\max} = 7$ and by extrapolating its dependence on $R_{\mathrm{MT}}G_{\max}$.

## II. FRACTIONAL AND INTEGER OCCUPANCIES OF KOHN-SHAM STATES

The obtained agreement in the total energies of silicon and chlorine among the considered three codes does not come out automatically. MADNESS and NWChem enforce integer occupation numbers of Kohn-Sham (KS) eigenstates and, thus, place the unoccupied $3p_z$ state below the doubly-degenerate $3p_x$ and $3p_y$ states. In contrast, our LAPW+lo implementation follows the common practice in computational solid-state physics, as it permits fractional occupancies and thus fills the energy levels according to Fermi-Dirac statistics, leading to a triple degeneracy of the $3p$ levels. This inconsistency between the codes is illustrated in Fig. 1. It results in different electron densities, and, hence, we obtain a discrepancy of $\sim 600$ $\mu$Ha for the total energy of silicon with respect to the MRA and LCAO. For the same reason, the total energies of the chlorine atom differ by $\sim 1200$ $\mu$Ha. However, as soon as integer occupancies of KS levels are introduced also in our LAPW+lo implementation, all methods yield consistent results as reported in Table 1 of the Letter.

Similar issues have to be addressed in calculations of NO and ClO. If fractional occupancies of KS levels are allowed, one obtains the lowest-energy solution for both molecules. However, in order to make the results obtained with **`exciting`**, MADNESS and NWChem consistent, integer occupancies must be enforced.

## III. COMPLETE-BASIS LIMIT IN GGA CALCULATIONS

This study relies solely on LSDA, however, high precision of LAPW+lo is not restricted to this exchange-correlation functional. To demonstrate it, we discuss how the total energy of oxygen atom reaches the complete-basis limit when the generalized-gradient approximation (GGA)[5] is used. The convergence behavior is summarized in Fig. 2. Similarly as in the LSDA case, a high-quality description of KS wavefunctions requires local orbitals with high angular momenta. The error in the total GGA energy is consistently higher than its LSDA counterpart at each considered $\ell_{\max}$. Nevertheless, a sub-$\mu$Ha error in the GGA calculation is achieved at $\ell_{\max} = 5$, LSDA requires $\ell_{\max} = 4$. Finally, we find no difference between the two exchange-correlation functionals in terms of convergence with respect to $R_{\mathrm{MT}}G_{\max}$.

To summarize, GGA does not present any new conceptual difficulties in comparison to LSDA. Furthermore, we

anticipate that the same conclusion will be true for any exchange-correlation functional, for which a local KS potential is available.

## IV. EQUATION OF STATE OF $\alpha$-IRON

Due to the ferromagnetic groundstate of $\alpha$-iron, the effective potential in the atomic spheres is substantially anisotropic. Therefore, we employ 4 $s$-, 4 $p$-, 3 $d$-, 4 $f$-, 5 $g$-, 5 $h$- and 4 $i$-type LOs for each $\ell m$ channel. Such a number of local orbitals is sufficient for reaching the 1-$\mu$Ha precision of the total energy for all considered atomic-sphere radii. This LO basis is used in the energy-versus-volume calculations in order to obtain equilibrium volume, bulk modulus, and its pressure derivative.

In the main paper, the Birch-Murnaghan equation of state has been applied. Here we show the results of a fit to a polynomial of sixth order in a range of volumes within ±10% around equilibrium. The results are summarized in Table VI. As these values depend on the chosen model for fitting the *ab initio* data, the obtained values differ somewhat from those reported in Table III of the Letter. However, the main conclusion remains unchanged, i.e., these quantities are extremely stable with respect to the choice of $R_{MT}$.

TABLE VI. Equilibrium volume, $V_0$, bulk modulus, $B_0$, and its pressure derivative, $B'$, for $\alpha$-iron as obtained from a fit to a sixth-degree polynomial. Calculations were performed using different atomic-sphere radii, $R_{MT}$ (in atomic units), and the LAPW cutoff parameter $R_{\mathrm{MT}}G_{\mathrm{max}} = 14$. The results were obtained from LSDA calculation using non-relativistic theory.

| $R_{MT}$ [a.u.] | $V_0$ [a.u.] | $B_0$ [GPa] | $B'$ |
|---|---|---|---|
| 1.4 | 71.3304 | 236.492 | 4.5552 |
| 1.5 | 71.3304 | 236.495 | 4.5551 |
| 1.6 | 71.3304 | 236.491 | 4.5552 |
| 1.7 | 71.3305 | 236.491 | 4.5552 |
| 1.8 | 71.3305 | 236.492 | 4.5553 |
| 1.9 | 71.3305 | 236.490 | 4.5551 |
| 2.0 | 71.3306 | 236.492 | 4.5549 |
| 2.1 | 71.3307 | 236.492 | 4.5555 |

Practical studies typically go beyond the LSDA and non-relativistic treatment of electrons. Hence, we study the behavior of various exchange-correlation functionals in scalar-relativistic calculations. The obtained results are summarized in Fig. 3 and Tab. VII. In all cases, the Brillouin zone is sampled using the Γ-centered $96 \times 96 \times 96$ grid. The LAPW cutoff parameter $R_{\mathrm{MT}}G_{\mathrm{max}}$ is in the range of 12–14. According to Tab. III of the main paper, such a choice ensures extremely robust total energies leading to converged parameters of the equation of state.

Fig. 3 provides an insight how the experimental and computational uncertainties as well as differences among various exchange-correlation functionals compare one to another. The PBE data from Refs.[6,7] are substantially scattered due to the diversity of methods and implementations applied in these calculations. In case none of them is picked as a reference, the PBE parametrisation of GGA yields the lattice constant and the bulk modulus of $\alpha$-iron with an uncertainty that is larger than the experimental one. This computational uncertainty is also greater than the difference between the results obtained in our high-precision calculations with PBEsol and AM05.The same conclusion holds for PW91 and PBE as well as acPBE and revPBE. In other words, a comparison of two GGAs may be be exceptionally tricky without high-precision tools at hand.

Finally, we point out that the lattice constants and the bulk moduli obtained with a range of exchange-correlation functionals follow a trend. A linear fit is shown in Fig. 3, and, curiously, it passes through a number of experimental data points. While we refrain from speculating on the physical meaning of this observation, it must be noted that this trend cannot be spotted based on calculations with the uncertainty as large as that in the recent PBE data[6,7].


[1] A. Gulans, S. Kontur, C. Meisenbichler, D. Nabok, P. Pavone, S. Rigamonti, S. Sagmeister, U. Werner, and C. Draxl, J. Phys.: Condens. Matter **26**, 363202 (2014).

[2] M. Valiev, E. Bylaska, N. Govind, K. Kowalski, T. Straatsma, H. V. Dam, D. Wang, J. Nieplocha, E. Apra, T. Windus, and W. de Jong, Comp. Phys. Comm. **181**, 1477 (2010).

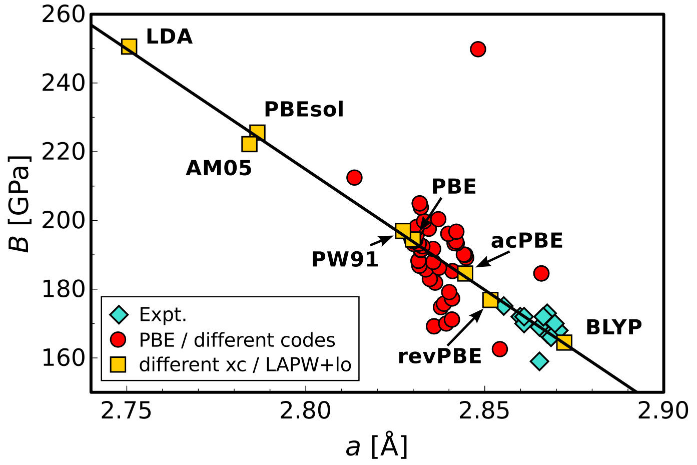


FIG. 3. Bulk moduli and lattice constants of $\alpha$-iron obtained in experiments[8–20], scalar-relativistic PBE calculations[6,7] using a variety of electronic structure codes and present scalar-relativistic calculations employing the LAPW+lo basis and various exchange-correlation functionals.

TABLE VII. Equilibrium volume, $V_0$, bulk modulus, $B_0$, and its pressure derivative, $B'$, for $\alpha$-iron as obtained from a fit to the Birch-Murnaghan equation of state. Calculations were performed using scalar-relativistic theory and different exchange-correlation functionals.

| | $V_0$ [a.u.] | $B_0$ [GPa] | $B'$ |
|---|---|---|---|
| LDA[4,21] | 70.2209 | 250.592 | 4.590 |
| PBE[5] | 76.4718 | 194.482 | 5.281 |
| PBEsol[22] | 73.0047 | 225.561 | 4.699 |
| PW91[23] | 76.2494 | 196.940 | 5.202 |
| revPBE[24] | 78.2374 | 176.860 | 5.435 |
| acPBE[25] | 77.6602 | 184.564 | 5.383 |
| BLYP[26,27] | 79.9444 | 164.056 | 5.904 |
| AM05[28] | 72.8261 | 222.210 | 4.812 |


[3] D. E. Woon and T. H. D. Jr., J. Chem. Phys. **98**, 13581371 (1993), http://dx.doi.org/10.1063/1.464303.
[4] J. P. Perdew and Y. Wang, Phys. Rev. B **45**, 13244 (1992).
[5] J. P. Perdew, K. Burke, and M. Ernzerhof, Phys. Rev. Lett. **77**, 3865 (1996).
[6] K. Lejaeghere, G. Bihlmayer, T. Björkman, P. Blaha, S. Blügel, V. Blum, D. Caliste, I. E. Castelli, S. J. Clark, A. Dal Corso, S. de Gironcoli, T. Deutsch, J. K. Dewhurst, I. Di Marco, C. Draxl, M. Dułak, O. Eriksson, J. A. Flores-Livas, K. F. Garrity, L. Genovese, P. Giannozzi, M. Giantomassi, S. Goedecker, X. Gonze, O. Grånäs, E. K. U. Gross, A. Gulans, F. Gygi, D. R. Hamann, P. J. Hasnip, N. A. W. Holzwarth, D. Iuşan, D. B. Jochym, F. Jollet, D. Jones, G. Kresse, K. Koepernik, E. Küçükbenli, Y. O. Kvashnin, I. L. M. Locht, S. Lubeck, M. Marsman, N. Marzari, U. Nitzsche, L. Nordström, T. Ozaki, L. Paulatto, C. J. Pickard, W. Poelmans, M. I. J. Probert, K. Refson, M. Richter, G.-M. Rignanese, S. Saha, M. Scheffler, M. Schlipf, K. Schwarz, S. Sharma, F. Tavazza, P. Thunström, A. Tkatchenko, M. Torrent, D. Vanderbilt, M. J. van Setten, V. Van Speybroeck, J. M. Wills, J. R. Yates, G.-X. Zhang, and S. Cottenier, Science **351**, aad3000 (2016).
[7] Delta calculation package, `https://molmod.ugent.be/deltacodesdft`.
[8] H. L. Zhang, S. Lu, M. P. J. Punkkinen, Q.-M. Hu, B. Johansson, and L. Vitos, Phys. Rev. B **82**, 132409 (2010).
[9] J. A. Rayne and B. S. Chandrasekhar, Phys. Rev. **122**, 1714 (1961).
[10] C. Rotter and C. S. Smith, Journal of Physics and Chemistry of Solids **27**, 267 (1966).
[11] J. Leese and A. E. L. Jr., Journal of Applied Physics **39**, 3986 (1968), https://doi.org/10.1063/1.1656884.
[12] G. Simmons and H. Wang, "Single crystal elastic constants and calculated aggregate properties," (MIT Press, Cambridge, Mass., 1971) Chap. Unified theory of exchange and correlation beyond the local density approximation, pp. 11–20.
[13] D. Dever, Journal of Applied Physics **43**, 3293 (1972), https://doi.org/10.1063/1.1661710.
[14] A. P. Jephcoat, H. K. Mao, and P. M. Bell, Journal of Geophysical Research: Solid Earth **91**, 4677 (1986).
[15] G. Ghosh and G. Olson, Acta Materialia **50**, 2655 (2002).
[16] S. Klotz and M. Braden, Phys. Rev. Lett. **85**, 3209 (2000).
[17] J. J. Adams, D. S. Agosta, R. G. Leisure, and H. Ledbetter, Journal of Applied Physics **100**, 113530 (2006),

http://aip.scitation.org/doi/pdf/10.1063/1.2365714.
[18] G. R. Speich, A. J. Schwoeble, and W. C. Leslie, Metallurgical Transactions **3**, 2031 (1972).
[19] M. Acet, H. Zähres, E. F. Wassermann, and W. Pepperhoff, Phys. Rev. B **49**, 6012 (1994).
[20] K. Lejaeghere, V. van Speybroeck, G. van Oost, and S. Cottenier, Critical Reviews in Solid State and Materials Sciences **39**, 1 (2014), http://dx.doi.org/10.1080/10408436.2013.772503.
[21] D. M. Ceperley and B. J. Alder, Phys. Rev. Lett. **45**, 566 (1980).
[22] J. P. Perdew, A. Ruzsinszky, G. I. Csonka, O. A. Vydrov, G. E. Scuseria, L. A. Constantin, X. Zhou, and K. Burke, Phys. Rev. Lett. **100**, 136406 (2008).
[23] J. Perdew, "Electronic structure of solids '91," (Akademie Verlag, Berlin, 1991) Chap. Unified theory of exchange and correlation beyond the local density approximation, pp. 11–20.
[24] Y. Zhang and W. Yang, Phys. Rev. Lett. **80**, 890 (1998).
[25] K. Burke, A. Cancio, T. Gould, and S. Pittalis, arXiv:0902.0885 [cond-mat.mtrl-sci].
[26] A. D. Becke, Phys. Rev. A **38**, 3098 (1988).
[27] C. Lee, W. Yang, and R. G. Parr, Phys. Rev. A **37**, 785 (1988).
[28] R. Armiento and A. E. Mattsson, Phys. Rev. B **72**, 085108 (2005).
